# Supplementary material for: SLayR: Scene Layout Generation with Rectified Flow
Source: arXiv:2412.05003 source file (2025-03-12)
Supplement: Supplementary file 1 [file main.tex]

\section{Ablation of Image Generators}
\label{sec:image_gen_ablation}
To control for the effect of the conditional generation component on our evaluation, we also run our text-to-image pipeline on competitors to InstanceDiffusion ~\cite{wang2024instancediffusioninstancelevelcontrolimage}, namely LMD+ ~\cite{lian2024llmgroundeddiffusionenhancingprompt},  GliGEN ~\cite{li2023gligenopensetgroundedtexttoimage}, and BoxDiff ~\cite{xie2023boxdifftexttoimagesynthesistrainingfree}, using the same image layouts we used in our main paper. 

We show the generated image metrics for LMD+ in ~\cref{tab:consolidated_table_metrics}. Like in our main paper, these metrics are inconclusive, and furthermore, the rankings of different layout generation methods differ depending on the downstream image generator.

\begin{table*}[ht]
\footnotesize
\newrobustcmd\B{\DeclareFontSeriesDefault[rm]{bf}{b}\bfseries}  
\def\Uline#1{#1\llap{\uline{\phantom{#1}}}}

\sisetup{detect-weight=true,
         mode=text,
         table-format=2.2,   
         add-integer-zero=false,
         table-space-text-post={*},
         table-align-text-post=false
         }

    \centering
        \rotatebox{90}{\textbf{LMD+}}
        \begin {tabular}{
        l
        S
        S
        S
        S
        S
        S
        S
        S
        S
        S
        S
        c   
        }
        \toprule
        \toprule
                % \multirow{2}{*}{\textbf{Model}} & LayoutT & LayoutT & GPT4o & GPT4o & Ours & ADE20K & ADE20K layouts \\
                % & (t=0) & (t=0.5) & & (COT) & & & halved \\
        {\textbf{Model}} & {\textbf{FID} ($\downarrow$)} & {\textbf{KID} ($10^{-2}$)($\downarrow$)} & {\textbf{CMMD} ($\downarrow$)} & {\textbf{IS} ($\uparrow$)} \\

        \midrule
        LayoutTransformer & \Uline{0.73} & 1.26 & 0.69 & \B{7.81}  \\
        \midrule
        GPT4o & 1.73 & \Uline{1.17} & 0.69 & \Uline{7.66}   \\
        \midrule
        Fixed Layout & 3.81 & 1.93 & 0.77 & 7.06  \\
        \midrule
        No Layout & 1.82 & 1.87 & 0.83 & 7.33  \\
        \midrule
        \rowcolor{lightgray}
        %Ours & 6.4 & 6.2 & 1.5 \\ Improved to
        \textbf{Ours} & \B 0.39 & \B 0.36 & \B 0.58 & 7.55 \\
        \bottomrule
        \bottomrule
        \end{tabular}
        
        \vspace{0.5cm}
        \rotatebox{90}{\textbf{GliGEN}}
        \begin {tabular}{
        l
        S
        S
        S
        S
        S
        S
        S
        S
        S
        S
        S
        c   
        }
        \toprule
        \toprule
        {\textbf{Model}} & {\textbf{FID} ($\downarrow$)} & {\textbf{KID} ($10^{-2}$)($\downarrow$)} & {\textbf{CMMD} ($\downarrow$)} & {\textbf{IS} ($\uparrow$)} \\

        \midrule
        LayoutTransformer & \B 0.66 & \B 0.45 & \Uline{0.61} & 8.02  \\
        \midrule
        GPT4o & 3.49 & 1.30 & 0.63 & \Uline{8.13}   \\
        \midrule
        Fixed Layout & 2.88 & 2.51 & 0.68 & 6.57  \\
        \midrule
        No Layout & 1.85 & 1.89 & 0.82 & 7.51 \\
        \midrule
        \rowcolor{lightgray}
        \textbf{Ours} & \Uline{1.65} & \Uline{0.46} & \B 0.50 & \B 8.28 \\
        \bottomrule
        \bottomrule
        
        \end{tabular}
        \vspace{0.5cm}
        
        \rotatebox{90}{\textbf{BoxDiff}}
        \begin {tabular}{
        l
        S
        S
        S
        S
        S
        S
        S
        S
        S
        S
        S
        c   
        }
        \toprule
        \toprule
        {\textbf{Model}} & {\textbf{FID} ($\downarrow$)} & {\textbf{KID} ($10^{-2}$)($\downarrow$)} & {\textbf{CMMD} ($\downarrow$)} & {\textbf{IS} ($\uparrow$)} \\

        \midrule
        LayoutTransformer &  1.37 & \Uline{1.62} & 0.53 & \B 9.04  \\
        \midrule
        GPT4o & \Uline{1.23} & 1.77 & 0.63 & 7.40   \\
        \midrule
        Fixed Layout & 2.32 & \B 1.42 & \Uline{0.52} & 6.92  \\
        \midrule
        No Layout & 1.82 & 1.87 & 0.83 & 7.33 \\
        \midrule
        \rowcolor{lightgray}
        \textbf{Ours} & \B 0.92 & 1.65 & \B 0.48 & \Uline{7.77} \\
        \bottomrule
        \bottomrule
        
        \end{tabular}
    \caption{Metrics evaluated on {\lmdPlus}, GliGEN, and BoxDiff. 
    For LMD+, our method is lowest in FID and KID. Different from the results on the InstanceDiffusion-generated images shown in~\cref{tab:traditional_metric_comparison}, it is now also lowest in CMMD.
    For GliGEN, our method now performs second-best on FID and KID, but best on CMMD and IS. This is opposite to the results of InstanceDiffusion-generated images shown in~\cref{tab:traditional_metric_comparison}
    For BoxDiff, our method is lowest in FID, we are not the lowest in KID anymore. We now perform the best in CMMD and second best in IS, unlike in images generated from InstanceDiffusion. 
    }
    \label{tab:consolidated_table_metrics}
\end{table*}

We also run a human evaluation on the images from each of these three generators, shown in ~\cref{fig:scatter_plots_consolidated}. Although our results are not identical between image generation methods, there are several important commonalities across all four of these methods: our method is significantly more plausible than {\layoutTransformer}, and has significantly more variety than {\gptFourO} and No Layout. We even outperform {\gptFourO} in terms of plausibility for LMD+ and GliGEN. These results support that our method offers an effective balance between plausibility and variety, regardless of the choice of image generator. These also show that our human evaluation procedure can help control for the choice of image generator.

\begin{figure*}[ht]
    \centering
    \begin{tabular}{c c c}
        % First Column (Scatters)
        \includegraphics[width=0.3\textwidth]{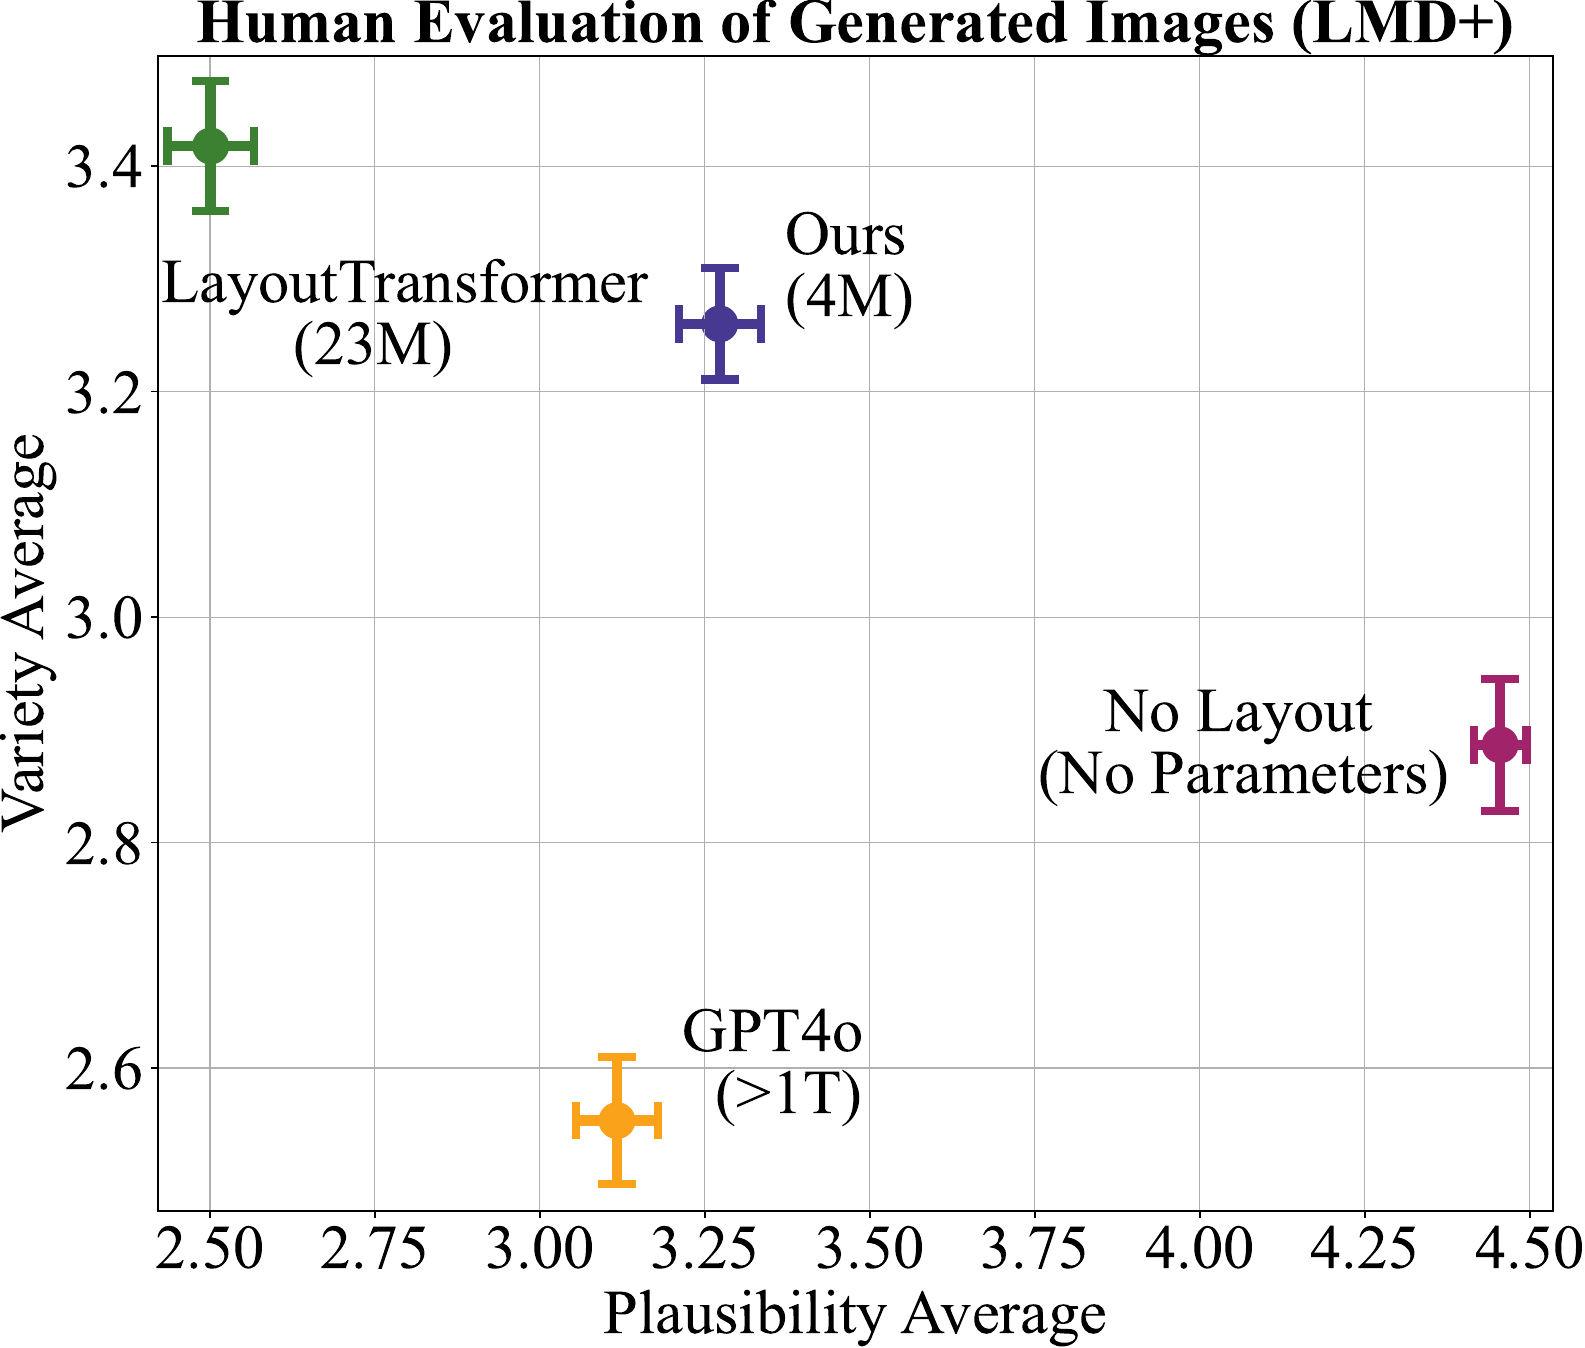} &
        \includegraphics[width=0.3\textwidth]{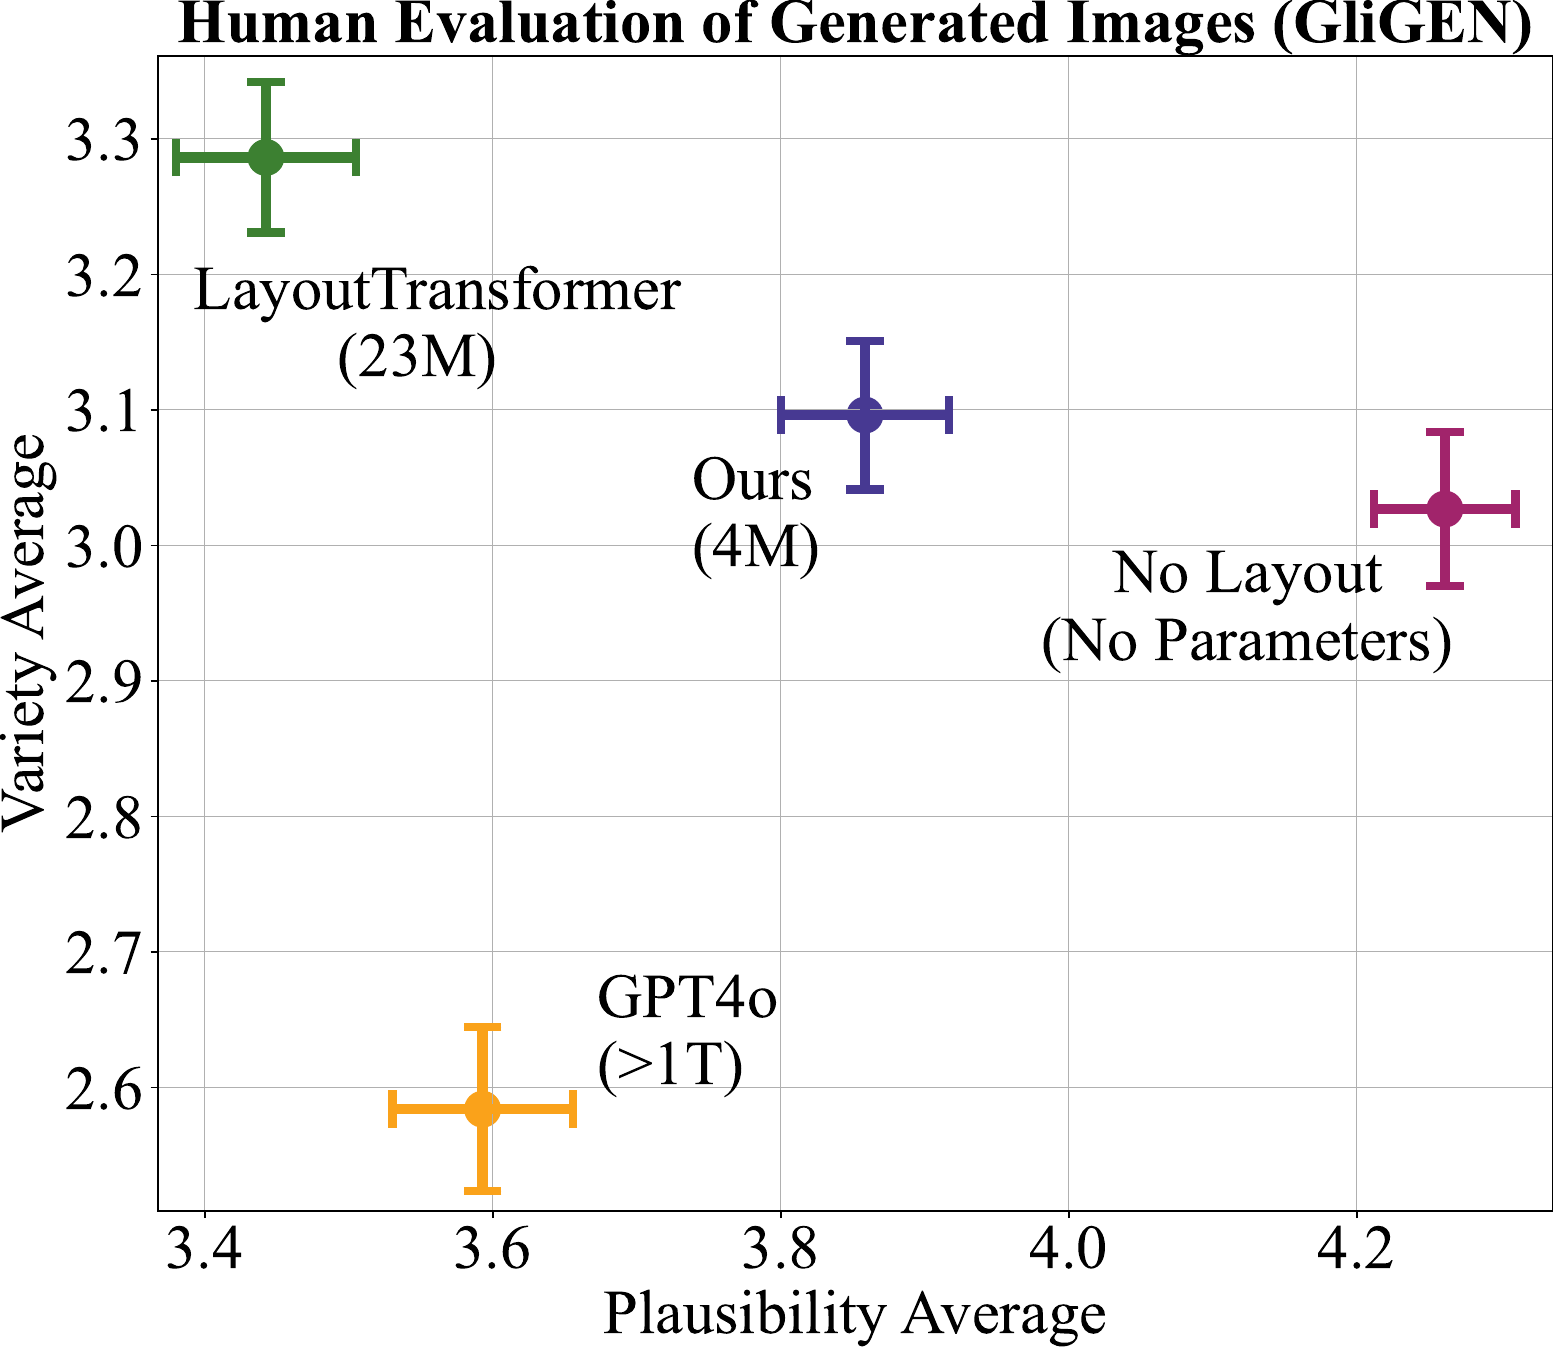} &
        \includegraphics[width=0.3\textwidth]{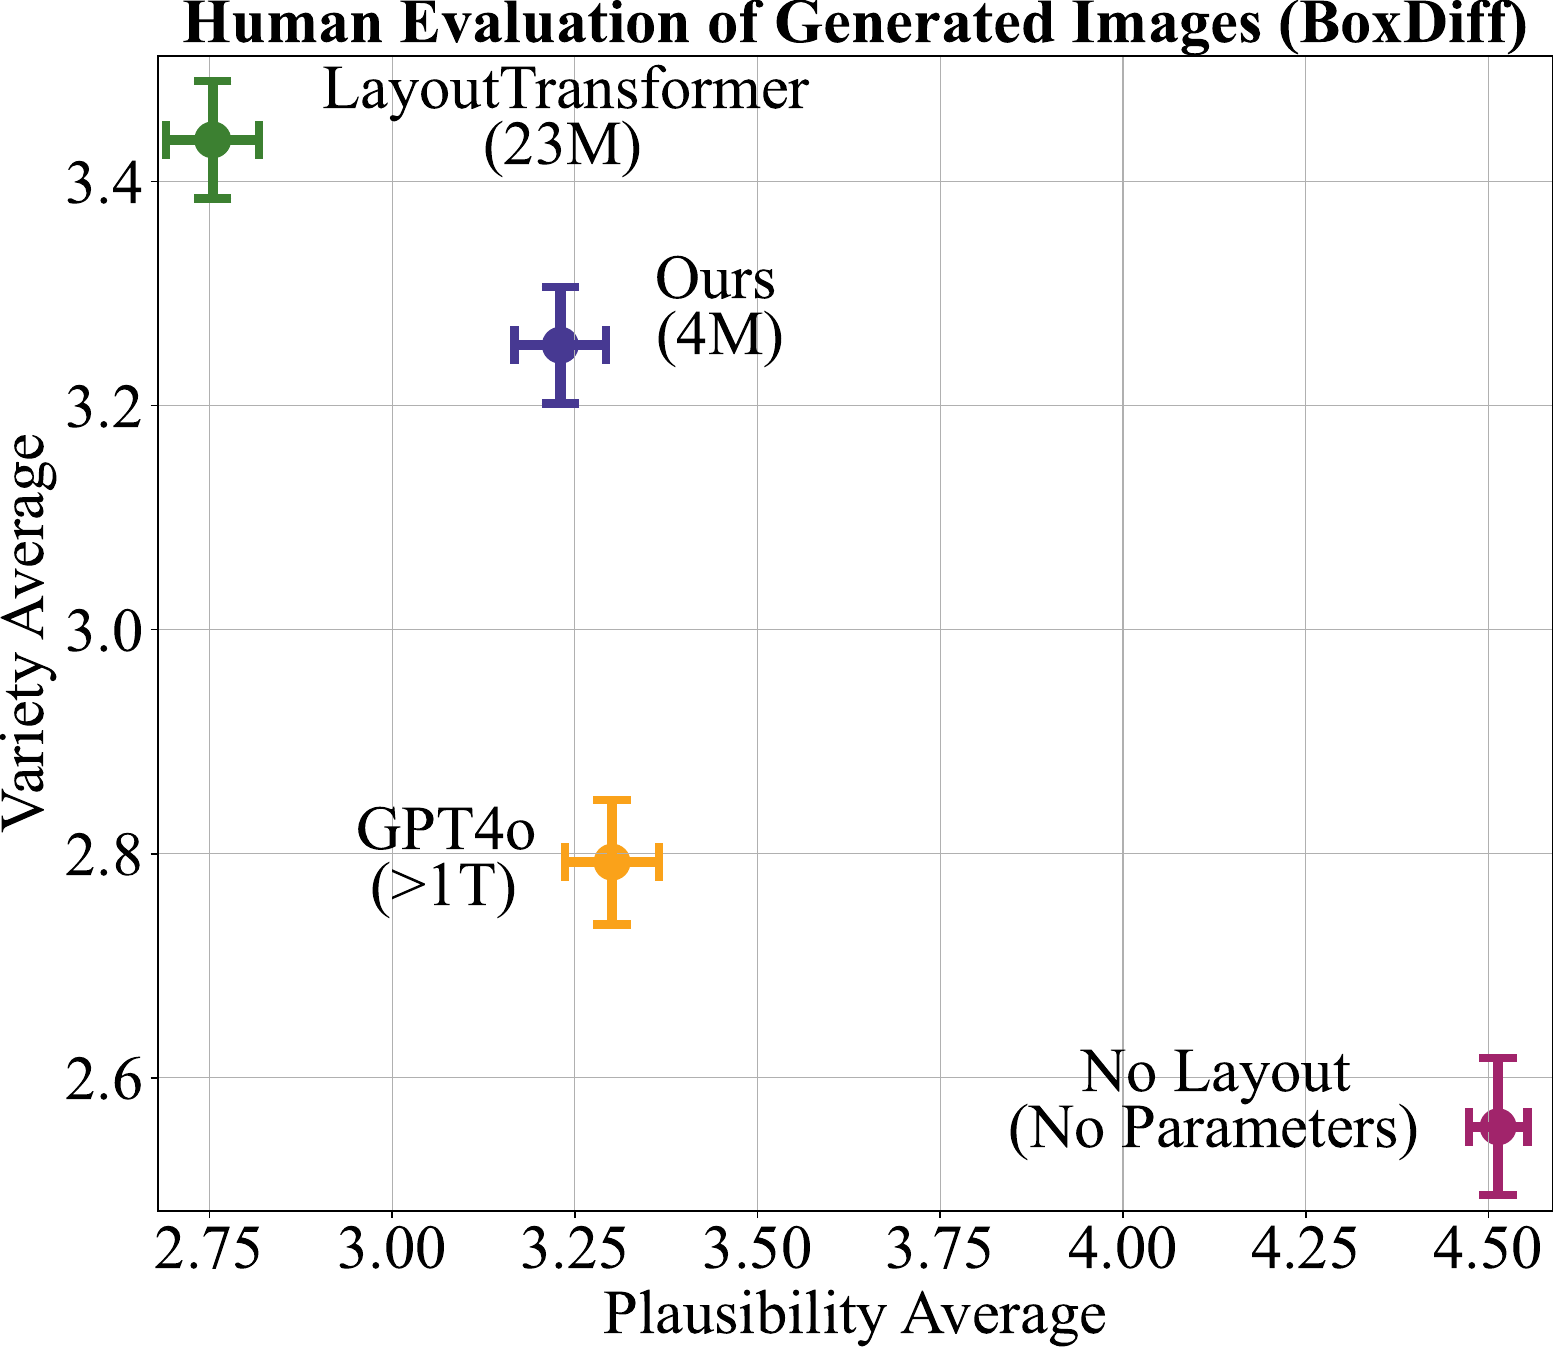} \\
    \end{tabular}
    \caption{Human evaluations of plausibility and variability of our pipeline using the {\lmdPlus}, GliGEN, and BoxDiff generators. Across these evaluators, we see that our method has higher plausibility than {\layoutTransformer}, and higher variety than {\gptFourO} and No Layout. In the case of {\lmdPlus} and GliGEN, we even have higher plausibility than {\gptFourO}}
    \label{fig:scatter_plots_consolidated}
\end{figure*}
