# Supplementary material for: SLayR: Scene Layout Generation with Rectified Flow
Source: arXiv:2412.05003 source file (2025-03-12)
Supplement: Supplementary file 2 [file consolidated_gen_ablation_figure.tex]

\begin{figure*}[ht]
    \centering
    \begin{tabular}{c c c}
        % First Column (Scatters)
        \includegraphics[width=0.3\textwidth]{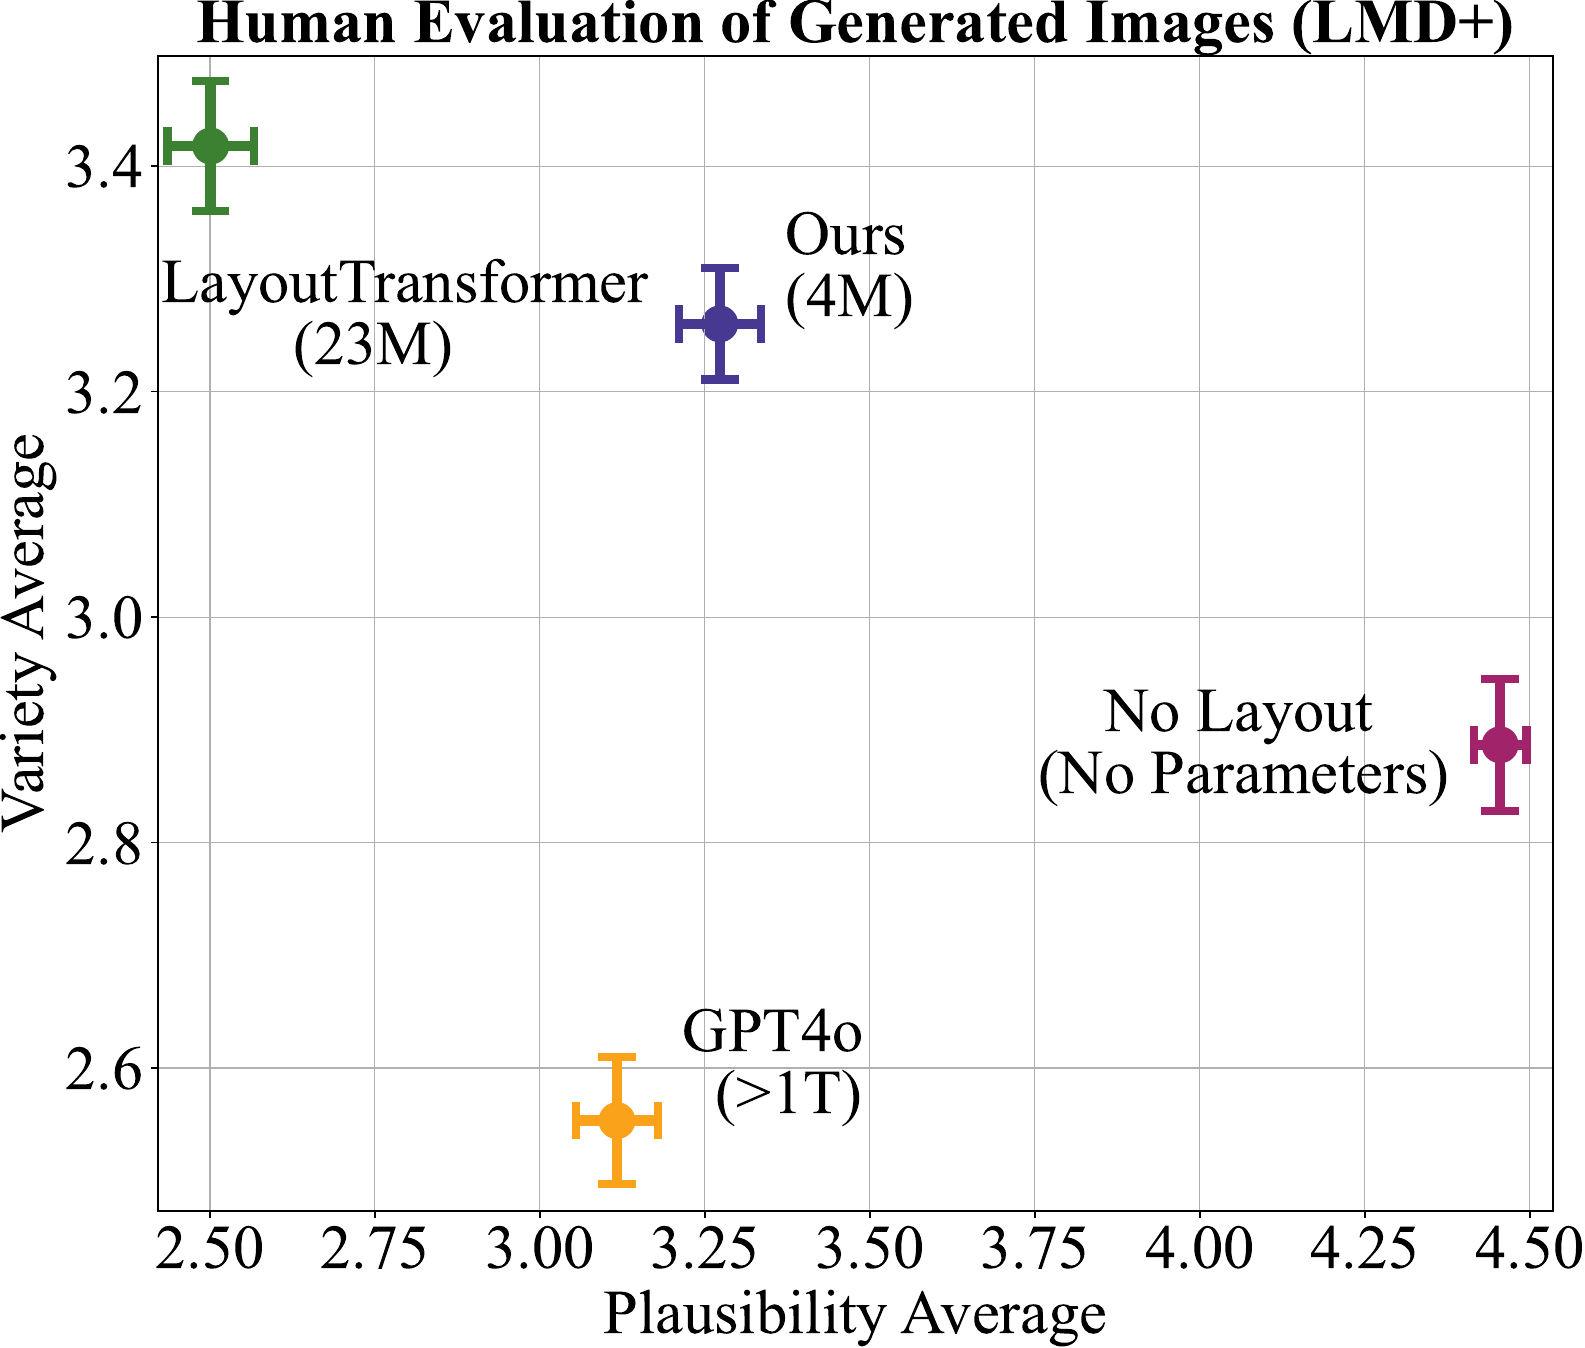} &
        \includegraphics[width=0.3\textwidth]{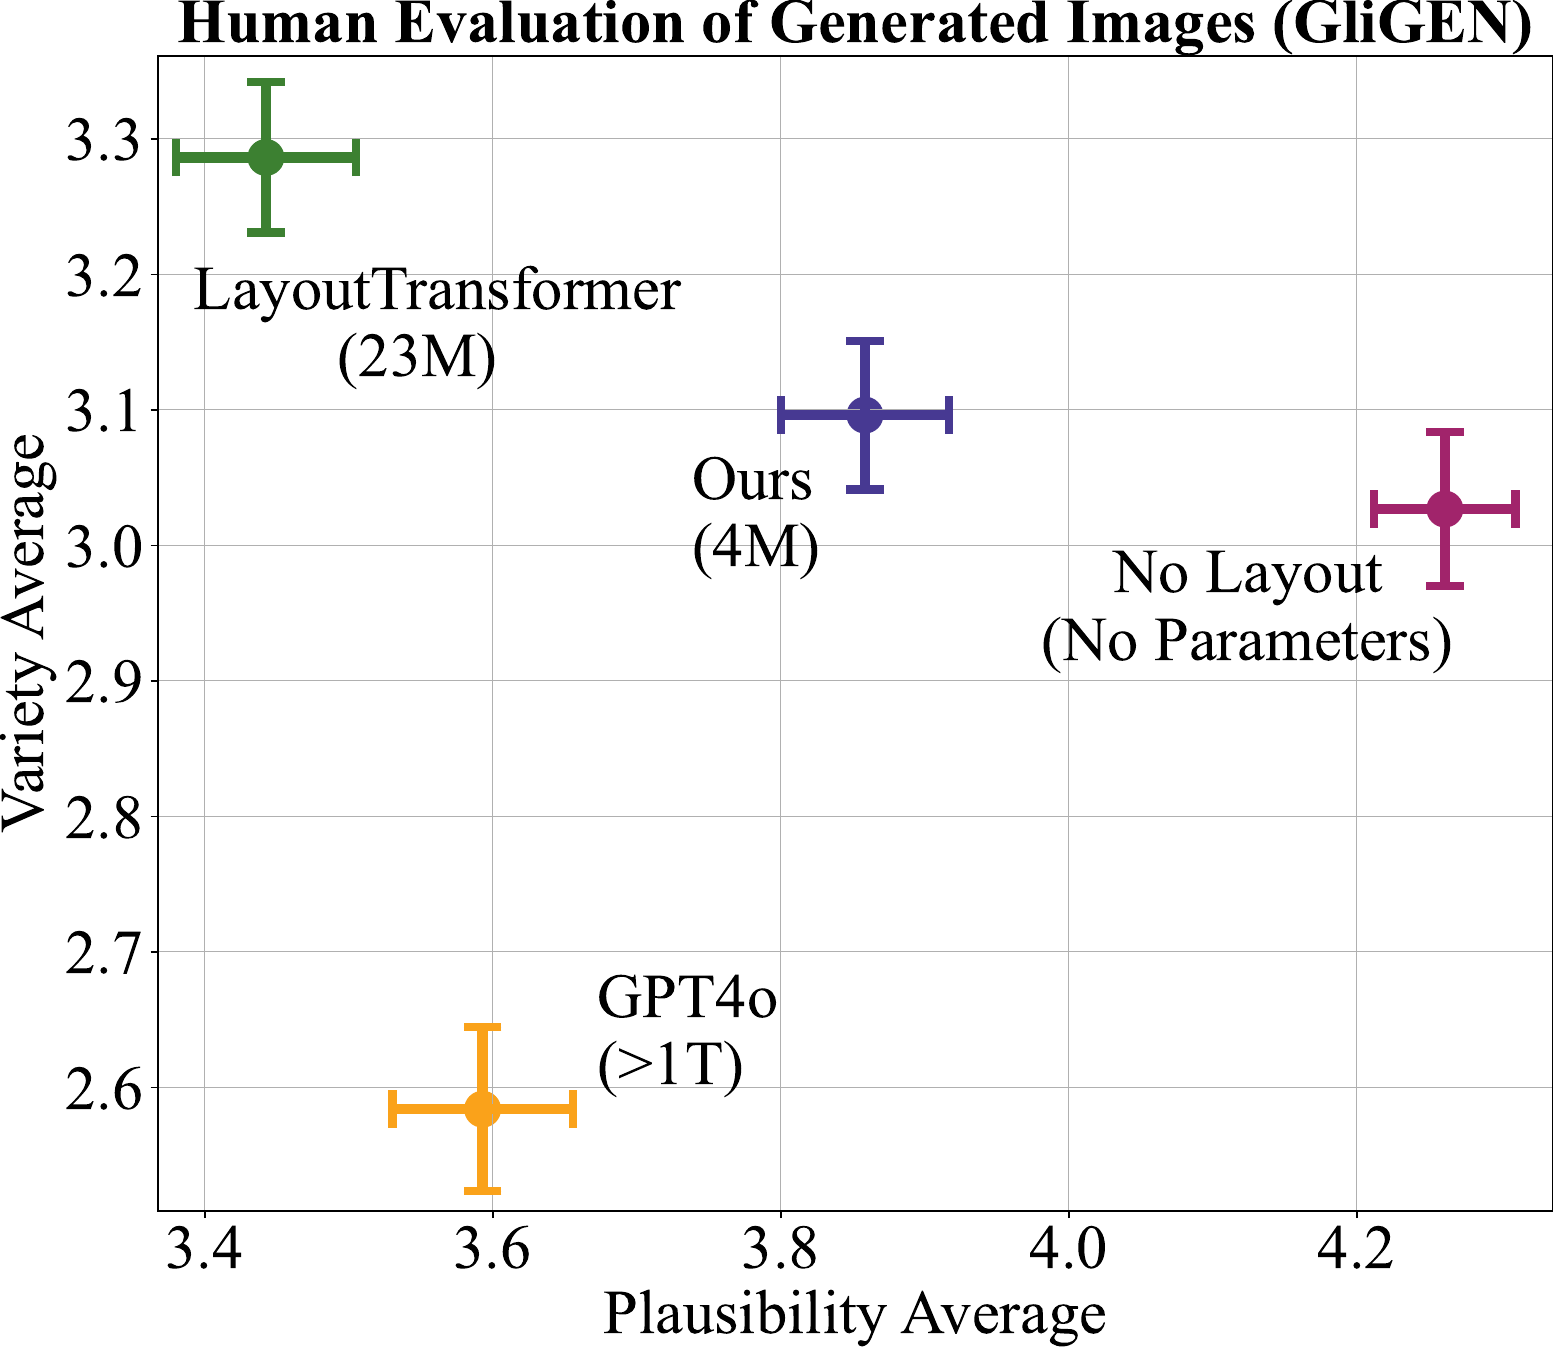} &
        \includegraphics[width=0.3\textwidth]{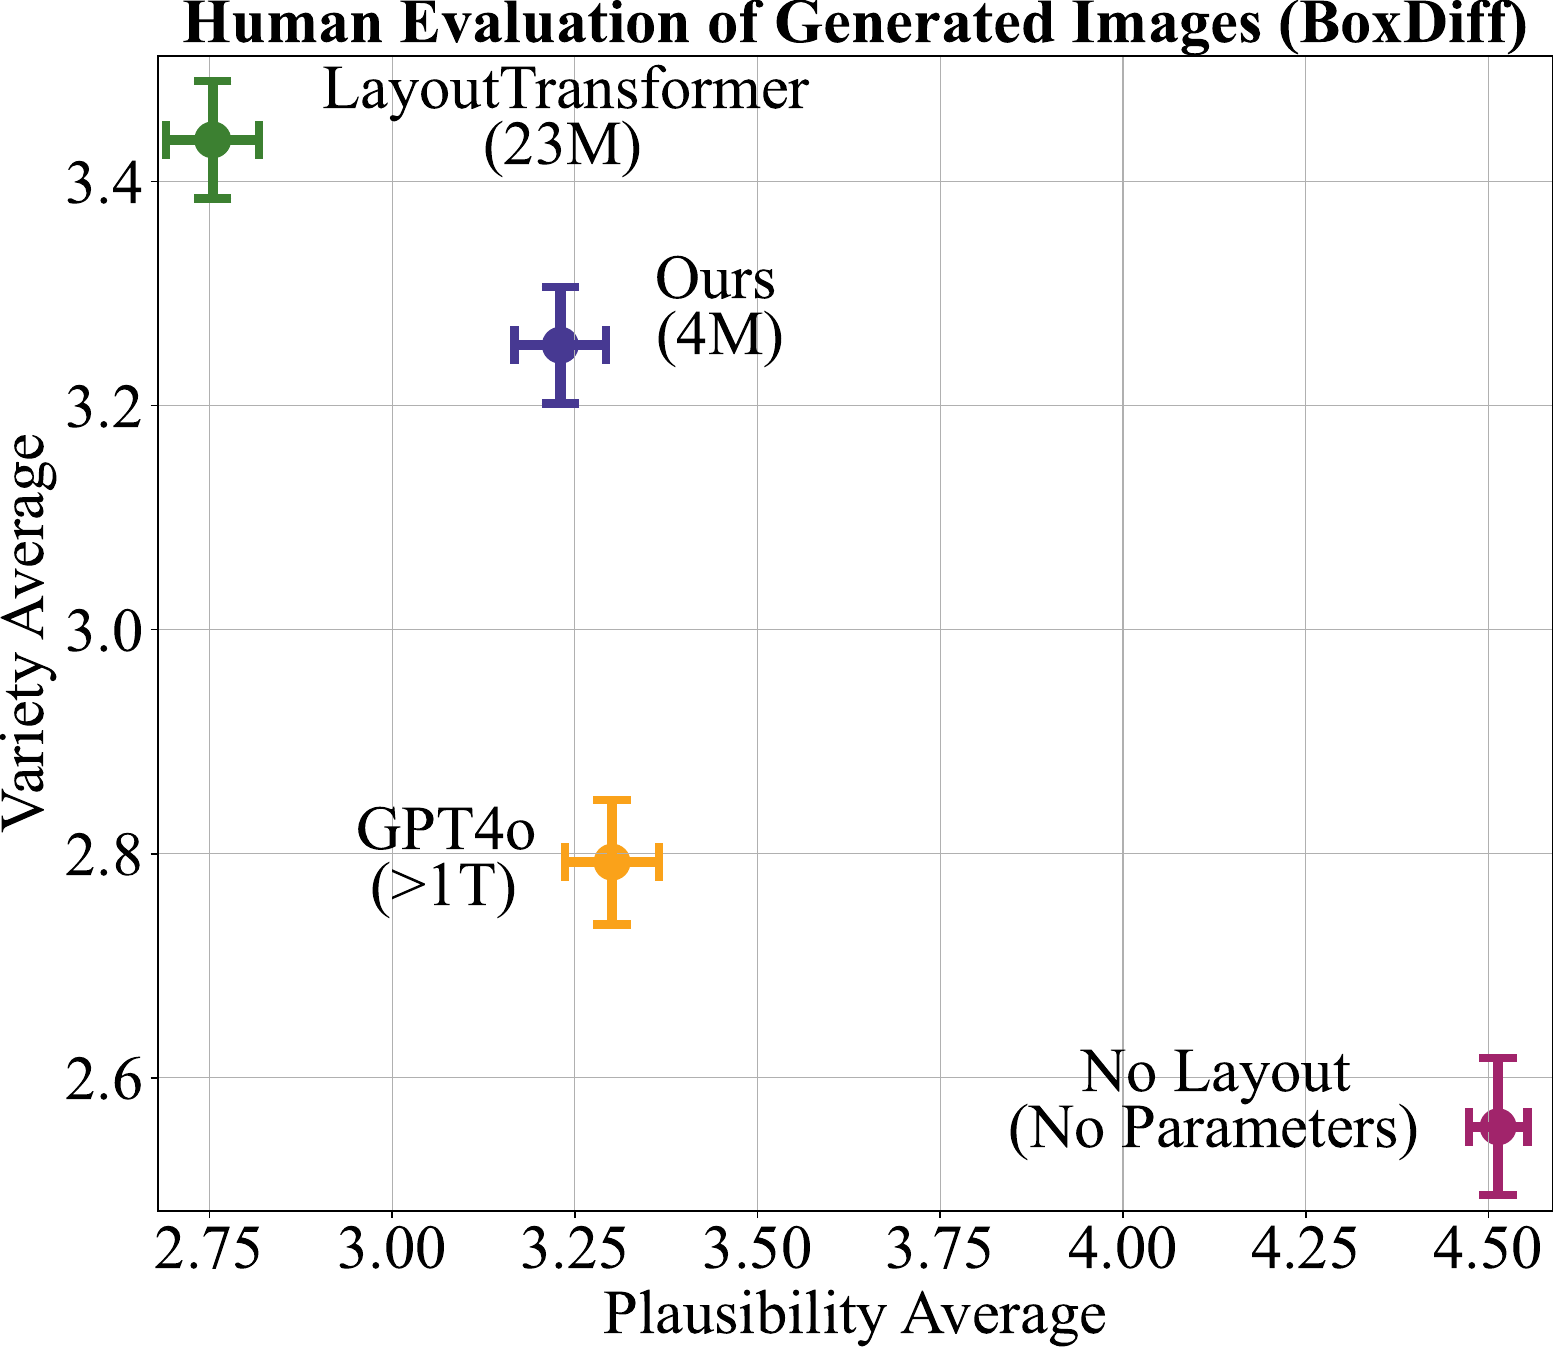} \\
    \end{tabular}
    \caption{Human evaluations of plausibility and variability of our pipeline using the {\lmdPlus}, GliGEN, and BoxDiff generators. Across these evaluators, we see that our method has higher plausibility than {\layoutTransformer}, and higher variety than {\gptFourO} and No Layout. In the case of {\lmdPlus} and GliGEN, we even have higher plausibility than {\gptFourO}}
    \label{fig:scatter_plots_consolidated}
\end{figure*}
