# Supplementary material for: SLayR: Scene Layout Generation with Rectified Flow
Source: arXiv:2412.05003 source file (2025-03-12)
Supplement: Supplementary file 3 [file consolidated_table.tex]

\begin{table*}[ht]
\footnotesize
\newrobustcmd\B{\DeclareFontSeriesDefault[rm]{bf}{b}\bfseries}  
\def\Uline#1{#1\llap{\uline{\phantom{#1}}}}

\sisetup{detect-weight=true,
         mode=text,
         table-format=2.2,   
         add-integer-zero=false,
         table-space-text-post={*},
         table-align-text-post=false
         }

    \centering
        \rotatebox{90}{\textbf{LMD+}}
        \begin {tabular}{
        l
        S
        S
        S
        S
        S
        S
        S
        S
        S
        S
        S
        c   
        }
        \toprule
        \toprule
                % \multirow{2}{*}{\textbf{Model}} & LayoutT & LayoutT & GPT4o & GPT4o & Ours & ADE20K & ADE20K layouts \\
                % & (t=0) & (t=0.5) & & (COT) & & & halved \\
        {\textbf{Model}} & {\textbf{FID} ($\downarrow$)} & {\textbf{KID} ($10^{-2}$)($\downarrow$)} & {\textbf{CMMD} ($\downarrow$)} & {\textbf{IS} ($\uparrow$)} \\

        \midrule
        LayoutTransformer & \Uline{0.73} & 1.26 & 0.69 & \B{7.81}  \\
        \midrule
        GPT4o & 1.73 & \Uline{1.17} & 0.69 & \Uline{7.66}   \\
        \midrule
        Fixed Layout & 3.81 & 1.93 & 0.77 & 7.06  \\
        \midrule
        No Layout & 1.82 & 1.87 & 0.83 & 7.33  \\
        \midrule
        \rowcolor{lightgray}
        %Ours & 6.4 & 6.2 & 1.5 \\ Improved to
        \textbf{Ours} & \B 0.39 & \B 0.36 & \B 0.58 & 7.55 \\
        \bottomrule
        \bottomrule
        \end{tabular}
        
        \vspace{0.5cm}
        \rotatebox{90}{\textbf{GliGEN}}
        \begin {tabular}{
        l
        S
        S
        S
        S
        S
        S
        S
        S
        S
        S
        S
        c   
        }
        \toprule
        \toprule
        {\textbf{Model}} & {\textbf{FID} ($\downarrow$)} & {\textbf{KID} ($10^{-2}$)($\downarrow$)} & {\textbf{CMMD} ($\downarrow$)} & {\textbf{IS} ($\uparrow$)} \\

        \midrule
        LayoutTransformer & \B 0.66 & \B 0.45 & \Uline{0.61} & 8.02  \\
        \midrule
        GPT4o & 3.49 & 1.30 & 0.63 & \Uline{8.13}   \\
        \midrule
        Fixed Layout & 2.88 & 2.51 & 0.68 & 6.57  \\
        \midrule
        No Layout & 1.85 & 1.89 & 0.82 & 7.51 \\
        \midrule
        \rowcolor{lightgray}
        \textbf{Ours} & \Uline{1.65} & \Uline{0.46} & \B 0.50 & \B 8.28 \\
        \bottomrule
        \bottomrule
        
        \end{tabular}
        \vspace{0.5cm}
        
        \rotatebox{90}{\textbf{BoxDiff}}
        \begin {tabular}{
        l
        S
        S
        S
        S
        S
        S
        S
        S
        S
        S
        S
        c   
        }
        \toprule
        \toprule
        {\textbf{Model}} & {\textbf{FID} ($\downarrow$)} & {\textbf{KID} ($10^{-2}$)($\downarrow$)} & {\textbf{CMMD} ($\downarrow$)} & {\textbf{IS} ($\uparrow$)} \\

        \midrule
        LayoutTransformer &  1.37 & \Uline{1.62} & 0.53 & \B 9.04  \\
        \midrule
        GPT4o & \Uline{1.23} & 1.77 & 0.63 & 7.40   \\
        \midrule
        Fixed Layout & 2.32 & \B 1.42 & \Uline{0.52} & 6.92  \\
        \midrule
        No Layout & 1.82 & 1.87 & 0.83 & 7.33 \\
        \midrule
        \rowcolor{lightgray}
        \textbf{Ours} & \B 0.92 & 1.65 & \B 0.48 & \Uline{7.77} \\
        \bottomrule
        \bottomrule
        
        \end{tabular}
    \caption{Metrics evaluated on {\lmdPlus}, GliGEN, and BoxDiff. 
    For LMD+, our method is lowest in FID and KID. Different from the results on the InstanceDiffusion-generated images shown in~\cref{tab:traditional_metric_comparison}, it is now also lowest in CMMD.
    For GliGEN, our method now performs second-best on FID and KID, but best on CMMD and IS. This is opposite to the results of InstanceDiffusion-generated images shown in~\cref{tab:traditional_metric_comparison}
    For BoxDiff, our method is lowest in FID, we are not the lowest in KID anymore. We now perform the best in CMMD and second best in IS, unlike in images generated from InstanceDiffusion. 
    }
    \label{tab:consolidated_table_metrics}
\end{table*}
